# Supplementary material for: S2TA: Exploiting Structured Sparsity for Energy-Efficient Mobile CNN Acceleration
Source: arXiv:2107.07983 source file (2022-01-06)
Supplement: Supplementary file 1 [file appendix.tex]

\section*{Appendix}
\label{sec:appendix}

\begin{figure*}[t]
\centering
\includegraphics[width=.9\textwidth]{figs/rednet50v1-perf.png} 
\caption{
ResNet50V1 per-layer energy and latency.
%for INT8 (Table~\ref{tab:dap-training}). 
%Normalized to the layer $conv1$ as 1.0 for SA arch.  
Relative to the SA baseline, S2TA-W-DBB and S2TA-A/W-DBB energy saving are 10.1\% and 50.2\%, respectively, while the latency reductions are 35.9\% and 52.3\%, respectively.
\RED{Can we add FC layer?}
}
\label{fig:resnet_v1_layers}
\vspace{-10pt}
\end{figure*}

\begin{figure}[h]
\centering
\includegraphics[width=0.40\textwidth]{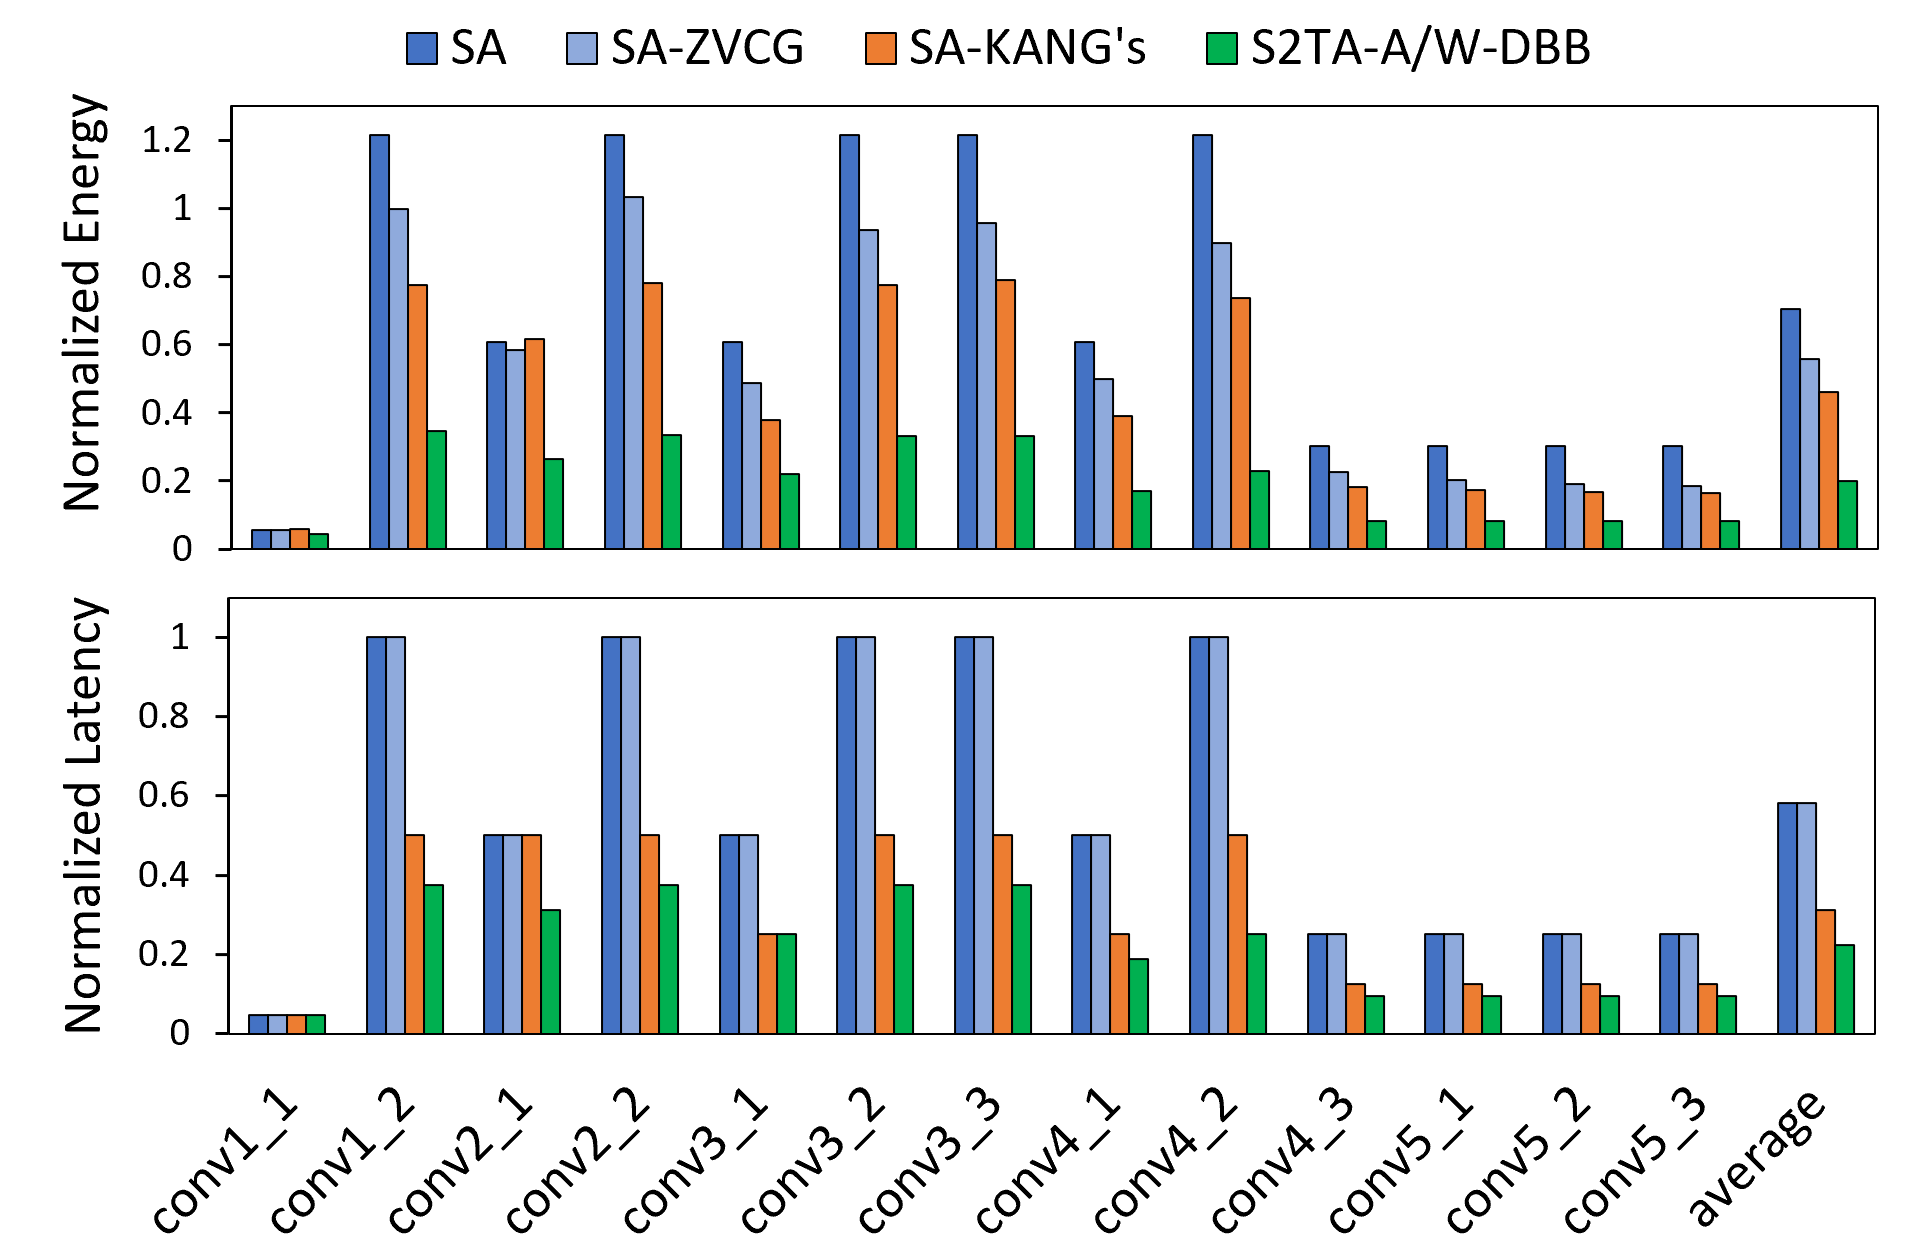}
\caption{
VGG16 per-layer energy and latency.
%4 TOPS nominal designs: normalized energy and latency for individual layers of INT8 VGG16 model. 
%Normalized to the layer $conv1\_2$ as 1.0 for SA arch. 
Relative to the SA baseline, S2TA-W-DBB shows an energy and latency reduction of 17.5\% and 46.4\%, respectively, while 
S2TA-A/W-DBB shows 64.1\% and 61.3\%, respectively.
}
\label{fig:vgg16_layers}
\vspace{-10pt}
\end{figure}

\begin{figure}[h]
\centering
\includegraphics[width=0.4\textwidth]{figs/mbv1-perf.png}
\caption{
MobileNetV1 per-layer energy and latency.
%4 TOPS nominal designs: normalized energy and latency for individual layers of INT8 MobileNet-v1 model in Table ~\ref{tab:dap-training}. 
%Normalized to the layer $conv2d\_0$ as 1.0 for SA arch.  
Relative to the baseline SA, the energy savings from S2TA-W-DBB and S2TA-A/W-DBB are 15.4\% and 43.6\%, respectively, while the latency reduction is 35.0\% and 40.3\%, respectively.  
\RED{for VGG, mobilenet and alexnet, instead of showing layers, do summary of overall energy/latency in one plot}
\RED{be careful with depthwise layers, which are slow and not shown here.. need to address this somehow}
}
\label{fig:mobilenet_layers}
\vspace{-1pt}
\end{figure}

\begin{figure}[h]
\centering
\includegraphics[width=0.43\textwidth]{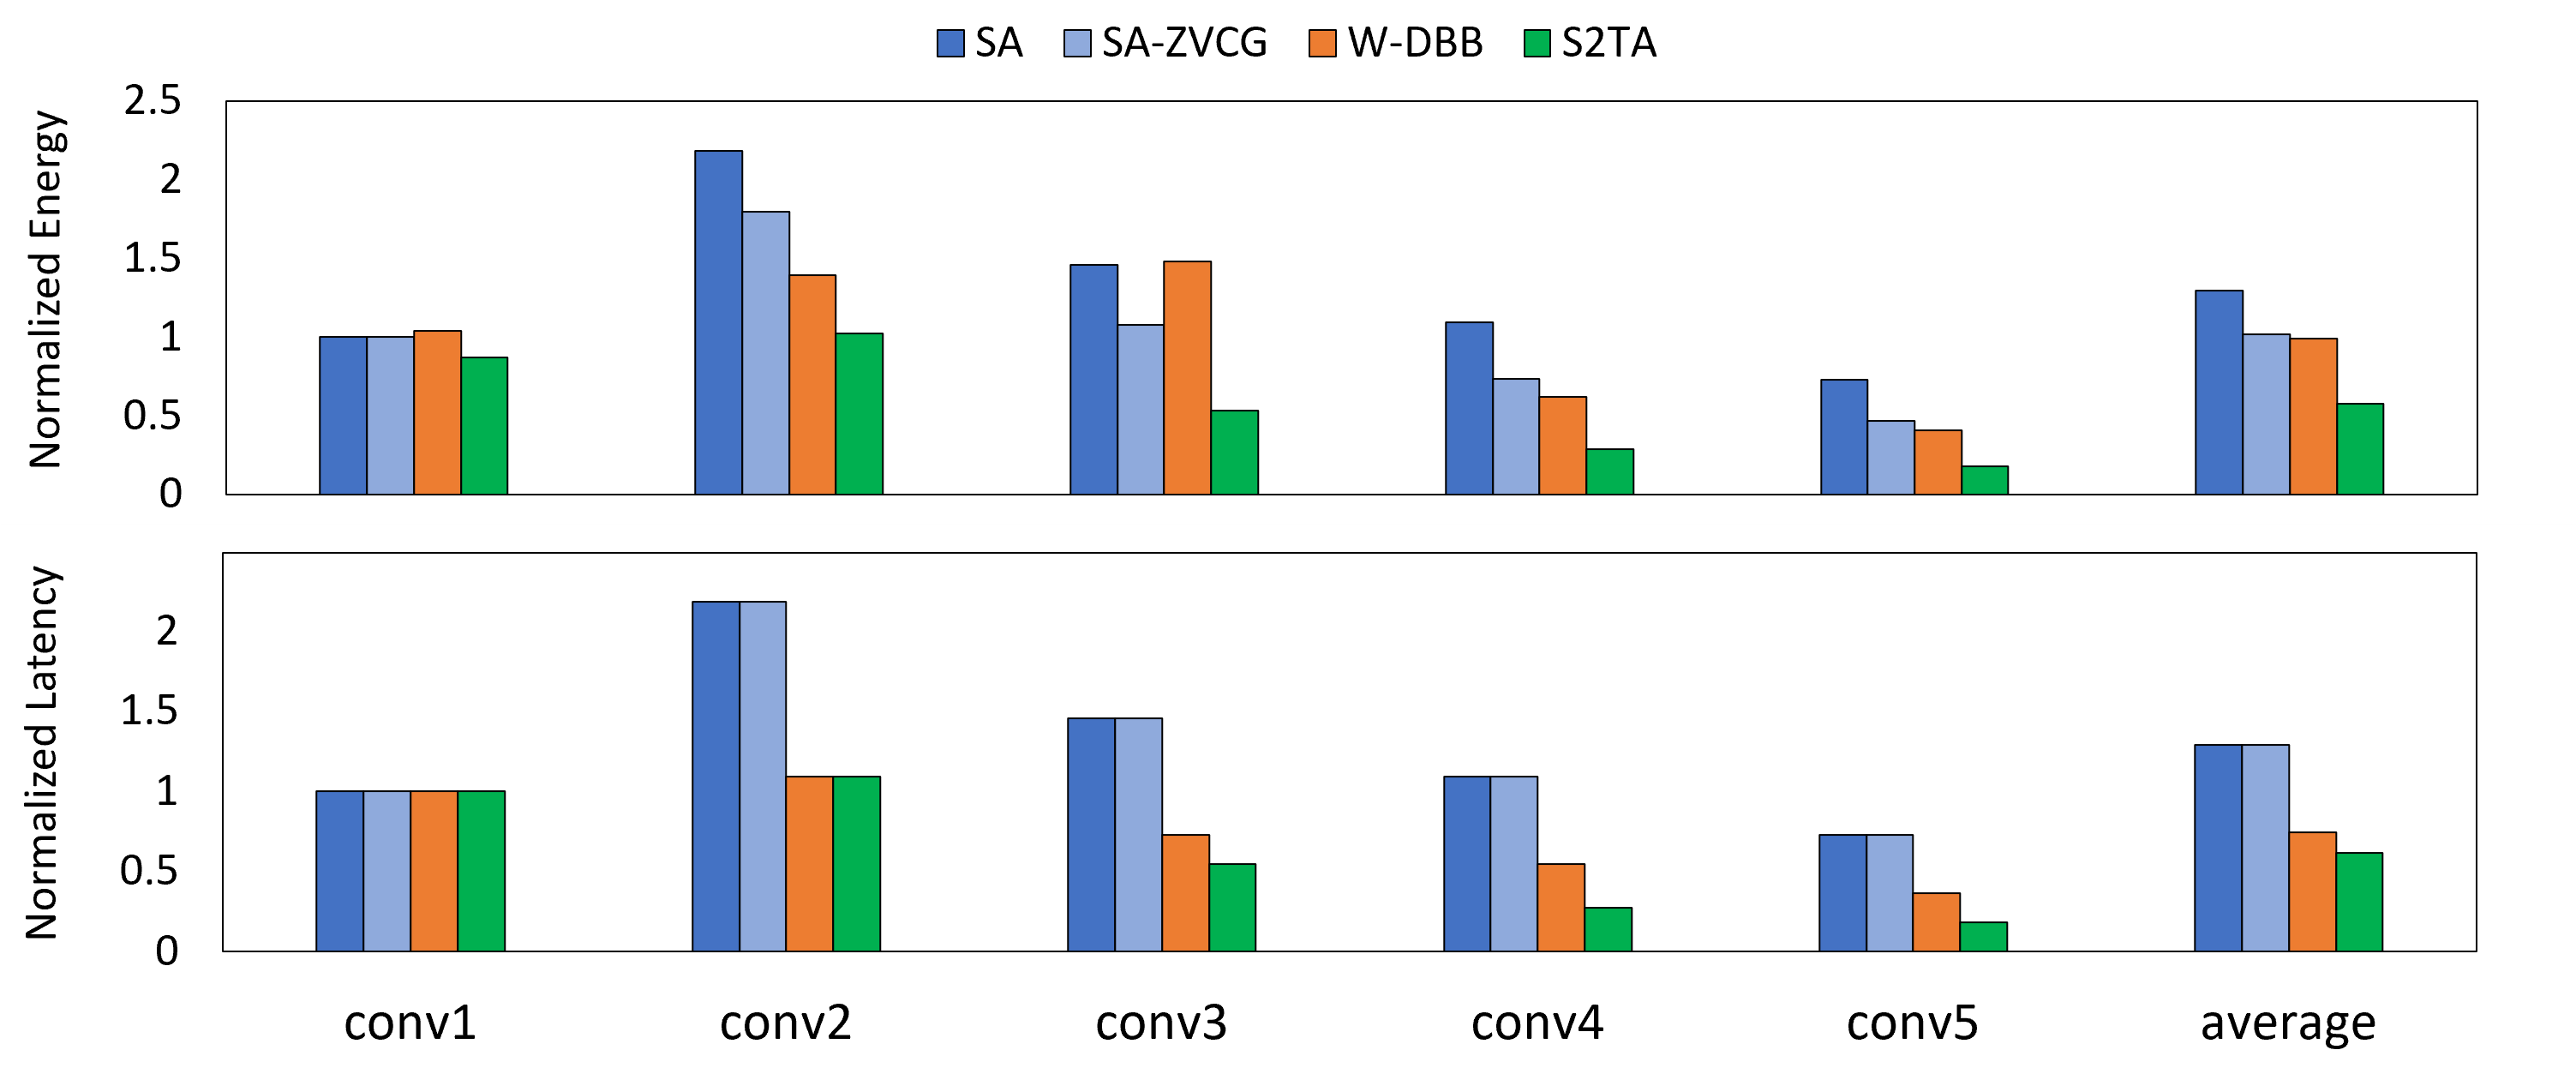}
\caption{
AlexNet per-layer energy and latency.
Relative to the baseline SA, the energy savings from S2TA-W-DBB and S2TA-A/W-DBB are 15.4\% and 43.6\%, respectively, while the latency reduction is 35.0\% and 40.3\%, respectively. }
\label{fig:mobilenet_layers}
\vspace{-1pt}
\end{figure}
